# Supplementary material for: Control of Competing Superconductivity and Charge Order by Non-equilibrium Currents
Source: arXiv:1804.09608 source file (2018-12-18)
Supplement: Supplementary file 1 [file suppl.pdf]

# Supplemental Material for 'Control of Competing Superconductivity and Charge Order by Non-equilibrium Currents'

Anne Matthies,[1] Jiajun Li,[1] and Martin Eckstein[1]

[1]*Department of Physics, University of Erlangen-Nürnberg, 91058 Erlangen, Germany*

## I. DMFT SETUP IN THE BETHE LATTICE

A Bethe lattice is an infinite connected graph with no loops, and coordination number $Z$. The Bethe lattice in the limit $Z \to \infty$ is widely used in DMFT model calculations, as it leads to a closed form of the self-consistency relation, and yields qualitatively correct results as far as the physics for a generic lattice is concerned [S1]. The results of the present work are therefore obtained for a Bethe lattice *with a scalar potential.* To ensure that the results are not specific to the Bethe lattice, the simulation has been repeated for a one-dimensional lattice, which also has a closed form of the self-consistency relation. The two simulations show qualitatively the same results and both confirm the main conclusion of the paper, namely the current-induced suppression of CDW. In these supplemental notes we derive the DMFT self-consistency relation for a Bethe lattice with a scalar potential gradient in the charge-density wave phase, and with a constant phase gradient in the superconducting phase.

### A. Bethe lattice with scalar potential

Due to the tree-like structure of the Bethe lattice, one can easily assign a scalar potential $V(z_j)$ to each site so that a lattice site with potential $V_0$ has half of its neighbors at potential $V_0 + V$ and the other half at $V_0 - V$, where $V = V(z_j + 1) - V(z_j)$. This is analogous to a cubic lattice in which the electric field is along the body-diagonal (111) direction: the six neighbors of site (0,0,0) are either in $+V$ direction $(1,0,0),(0,1,0),(0,0,1)$ or in $-V$ direction $(-1,0,0),(0,-1,0),(0,0,-1)$. Following the general derivation of the DMFT self-consistency from the cavity construction [S1], the DMFT self-consistency relation for the hybridization function $\Delta_o(\omega)$ at a lattice site $o$ is given by

$$\Delta_o(\omega) = \sum_p t_{op} G_p^{[o]}(\omega) t_{po} \tag{S1}$$

where the sum extends over all nearest neighbors of $o$, $t_{op}$ is the hopping from $o$ to $p$ ($t_{po} = t^*_{op}$), and $G_p^{[o]}(\omega)$ is the cavity Green's function, i.e., the Green's function at site $p$ with site $o$ excluded from the lattice. In the limit of infinite coordination number, the hopping is scaled as $t_{op} \propto Z^{-1/2}$ to maintain a finite bandwidth, and $G^{[o]}(\omega) = G_p(\omega)$. We use units such that $t_{op} = \sqrt{2}t_0/\sqrt{Z}$, where $t_0$ sets the energy scale. When $Z/2$ of the sites $p$ are at potential $+V$ and $-V$ compared to site $o$, respectively, the self-consistency therefore reduces to

$$\Delta_o(\omega) = \frac{(\sqrt{2}t_0)^2}{2}[G_{o,+}(\omega) + G_{o,-}(\omega)], \tag{S2}$$

where $G_{o,\pm}(\omega)$ is the Green function at neigboring sites with potential $\pm V$ with respect to $o$.

In the charge density wave phase (CDW) the bipartite Bethe lattice is divided into two sublattices $A$ and $B$. Furthermore, in an infinite lattice the Green's functions at two otherwise equivalent sites which differ only in the scalar potential are related by a shift in the frequency. Given the structure of a Bethe lattice, a central lattice site A (B) is connected to B (A) sites, with energy shift $-V$ $(+V)$ along a bond parallel (anti-parallel) to the electric field, as shown in FIG. S1. Hence, Eq. (S2) becomes

$$\Delta_{A(B)}(\omega) = \sum_\pm t_0^2 G_{B(A)}(\omega \pm V) = \sum_\pm \hat{F}^\pm_{A(B)}(\omega), \tag{S3}$$

which is the self-consistency stated in the main text.

### B. Superconducting phase

Contrary to the CDW phase, a constant bias leads to oscillating current in the superconducting phase due to AC Josephson effect, which is generally not expected in a bulk system. In the SC phase, the DC-current emerges

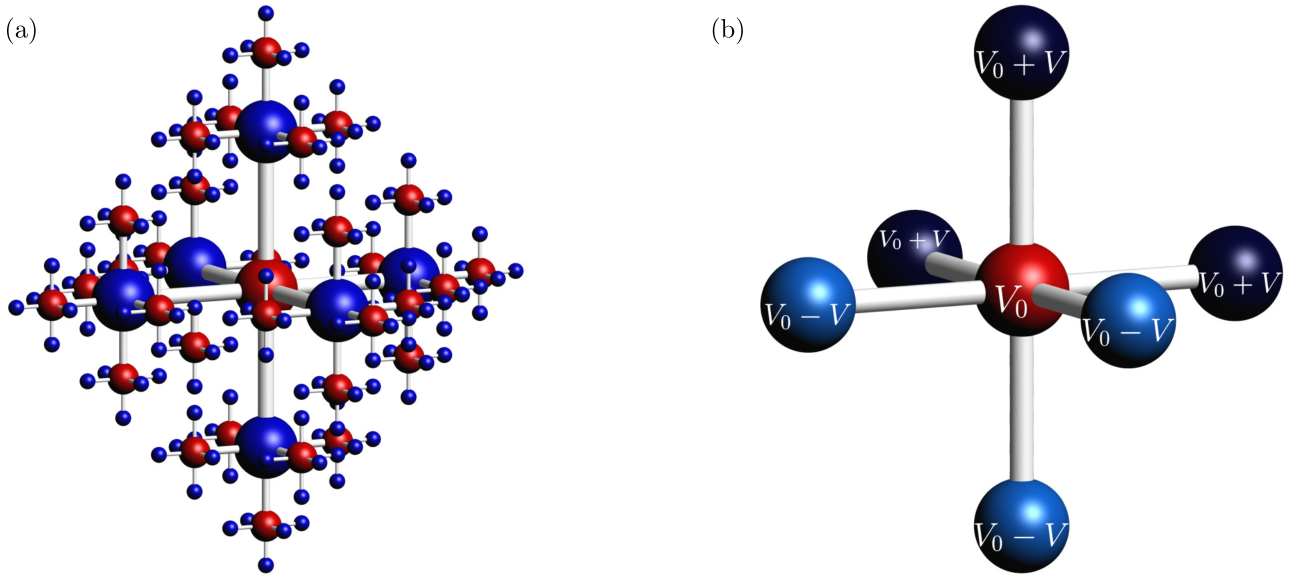


FIG. S1: Bethe lattice with coordination number $Z=6$. (a) The two sublattices A and B labeled with red and blue colors. (b) Zoom-in of (a) near the central site with different onsite potentials indicated by different colors.

due to a continuous phase twist of the order parameter along the direction of the DC-current. The Bethe lattice is described as in Sect. A, but no scalar potential is assigned. On the contrary, a phase twist $\phi$ is introduced for any two neighboring sites. With a gauge transformation, the phase twist is transformed into a phase factor in the hopping, $t_{op}=\sqrt{2}t_0 e^{\pm i\phi}/\sqrt{Z}$ in Eq. (S1). The self-consistent condition is then given by $\hat{F}^{\pm}_{A(B)}(\omega)=t_0^2\mathrm{e}^{\pm i\sigma_z\phi}G_{B(A)}(\omega)\mathrm{e}^{\mp i\sigma_z\phi}$, where both the hybridization functions $\hat{F}_{A(B)}$ and Green's functions $G_{B(A)}$ are understood as $2\times 2$ Nambu matrices and $\sigma_z$ is the Pauli matrix.

[S1] A. Georges, G. Kotliar, W. Krauth, and M. J. Rozenberg, Rev. Mod. Phys. **68**, 13 (1996).
